# Supplementary material for: Comparing Generic and Community-Situated Crowdsourcing for Data Validation in the Context of Recovery from Substance Use Disorders
Source: arXiv:2012.06965 source file (2020-12-13)
Supplement: Supplementary file 1 [file appendix.tex]

\appendix

\section{Geographic Analysis}\label{app:geo_analysis}

Test appendix section. Table \ref{app:tab:geo_full_model_comparison}.

% Table created by stargazer v.5.2.2 by Marek Hlavac, Harvard University. E-mail: hlavac at fas.harvard.edu
% Date and time: Fri, Dec 27, 2019 - 11:31:39 AM
\begin{table}[!htbp] \centering 
\begin{tabular}{@{\extracolsep{5pt}}lccc} 
%\\[-1.8ex]\hline 
%\hline \\[-1.8ex] 
\\[-1.8ex] & (1) & (2) & (3)\\ 
\hline \\[-1.8ex] 
 censored\_log(target\_outdegree, min = 1) & $-$0.191$^{***}$ & $-$0.225$^{***}$ & $-$0.231$^{***}$ \\ 
  & (0.005) & (0.025) & (0.029) \\ 
%  & & & \\ 
 target\_has\_indegree & 0.756$^{***}$ & 1.907$^{***}$ & 1.795$^{***}$ \\ 
  & (0.017) & (0.170) & (0.182) \\ 
%  & & & \\ 
 censored\_log(target\_indegree, min = 1) & 0.649$^{***}$ & 0.960$^{***}$ & 0.974$^{***}$ \\ 
  & (0.005) & (0.027) & (0.030) \\ 
%  & & & \\ 
 is\_reciprocal & 20.016$^{***}$ & 8.458$^{***}$ & 7.999$^{***}$ \\ 
  & (0.460) & (0.574) & (0.568) \\ 
%  & & & \\ 
 is\_weakly\_connected & 1.767$^{***}$ & 4.647$^{***}$ & 4.281$^{***}$ \\ 
  & (0.021) & (0.430) & (0.435) \\ 
%  & & & \\ 
 is\_friend\_of\_friend & 5.220$^{***}$ & 3.196$^{***}$ & 2.801$^{***}$ \\ 
  & (0.097) & (0.201) & (0.207) \\ 
%  & & & \\ 
 factor(target\_author\_type)mixed & 0.020 & 0.110 & 0.111 \\ 
  & (0.018) & (0.085) & (0.098) \\ 
%  & & & \\ 
 factor(target\_author\_type)p & $-$0.242$^{***}$ & $-$0.187$^{***}$ & $-$0.247$^{***}$ \\ 
  & (0.012) & (0.063) & (0.072) \\ 
%  & & & \\ 
 is\_author\_type\_shared & 0.299$^{***}$ & 0.331$^{***}$ & 0.295$^{***}$ \\ 
  & (0.012) & (0.059) & (0.068) \\ 
%  & & & \\ 
 is\_heh\_condition\_shared & 0.213$^{***}$ & 0.366$^{***}$ & 0.400$^{***}$ \\ 
  & (0.009) & (0.049) & (0.056) \\ 
%  & & & \\ 
 target\_is\_multisite\_author & 0.315$^{***}$ & 0.752$^{***}$ & 0.772$^{***}$ \\ 
  & (0.015) & (0.058) & (0.066) \\ 
%  & & & \\ 
 target\_is\_mixedsite\_author & 0.474$^{***}$ & 0.367$^{***}$ & 0.352$^{***}$ \\ 
  & (0.008) & (0.059) & (0.067) \\ 
%  & & & \\ 
 target\_update\_count & $-$0.0003$^{***}$ & $-$0.001$^{***}$ & $-$0.0004$^{***}$ \\ 
  & (0.00004) & (0.0001) & (0.0001) \\ 
%  & & & \\ 
 target\_update\_frequency & 0.007$^{***}$ & 0.013$^{***}$ & 0.013$^{***}$ \\ 
  & (0.0002) & (0.002) & (0.002) \\ 
%  & & & \\ 
 target\_days\_since\_most\_recent\_update & $-$0.011$^{***}$ & $-$0.006$^{***}$ & $-$0.005$^{***}$ \\ 
  & (0.00005) & (0.0001) & (0.0001) \\ 
%  & & & \\ 
 target\_days\_since\_first\_update & $-$0.001$^{***}$ & $-$0.001$^{***}$ & $-$0.0005$^{***}$ \\ 
  & (0.00001) & (0.00003) & (0.00004) \\ 
%  & & & \\ 
 is\_state\_assignment\_shared &  &  & 2.723$^{***}$ \\ 
  &  &  & (0.069) \\ 
%  & & & \\ 
\hline \\[-1.8ex] 
Observations & 155,141 & 7,007 & 7,007 \\ 
Log Likelihood & $-$133,746.600 & $-$4,830.810 & $-$3,743.011 \\ 
Test Accuracy & 77.2\% & 84.3\% & 87.1\% \\
%\hline 
\hline \\[-1.8ex] 
%\textit{Note:}  & \multicolumn{3}{r}{} \\ 
\end{tabular}
\caption{Multinomial logit models for initiation with the subset of authors given US state assignments via IP geolookup. Model (1) is the full model on all the initiations in the analysis period. Model (2) includes only the subset of authors with state assignments. Model (3) is that same subset with an additional dummy variable indicating matching state assignment between the initiator and the candidate. Comparing (1) and (2) demonstrates that this author subset is broadly similar in initiation factors compared to the full author sample, while (3) demonstrates the importance of matching state assignments.  Note that a matching state assignment is less important than the network-based features. \textit{Note:} $^{***}$ indicates p$<$0.01}
\label{app:tab:geo_full_model_comparison} 
\end{table} 

\begin{table}[]
    \centering
    \begin{tabular}{lrr}
Health-condition category & Count & \% \\ \hline
None & 152,818 & 42.17\% \\
Cancer & 109,339 & 30.18\% \\
Other & 37,556 & 10.36\% \\
Surgery/Transplantation & 15,415 & 4.25\% \\
Injury & 12,910 & 3.56\% \\
Cardiovascular/Stroke & 12,685 & 3.50\% \\
Neurological Condition & 9,376 & 2.59\% \\
Infant/Childbirth & 7,952 & 2.19\% \\
Condition Unknown & 2,252 & 0.62\% \\
Congenital/Immune Disorder & 2,042 & 0.56\% \\ \hline
    \end{tabular}
    \caption{Health condition assignments to valid authors.}
    \label{app:tab:health_condition_category_counts}
\end{table}

\input{init_timing_full_models}
